# Supplementary material for: Learning Mixtures of Unknown Causal Interventions
Source: arXiv:2411.00213 source file (2024-10-31)
Supplement: Supplementary file 1 [file psi_mec_imec_discussion.tex]

\section{Mixture-MEC = I-MEC for Linear SEM with Gaussian Noise}
\label{sec:mixture_mec}

Given observational distribution is known and we have access to interventional distribution on the unknown target set $U_k$, \citet{Squires2020UTGSP} gave necessary and sufficient conditions to identify the unknown intervention target $U_k$. \abhinav{Check if this condition is sufficient or not} Below we restate the condition formally:   
\abhinav{Define the notation for interventional distribution in section 2.}
\begin{assumption}[Direct $\mathcal{I}$-Faithfulness, Assumption 1 in \cite{Squires2020UTGSP}]
Given interventional distribution $f_{k}$ with intervention targets $U_{k}$, we assume that $f_{U_k}(x_i|\bm{x}_{Q}) \neq f_{\text{obs}}(x_i|\bm{x}_{Q})$ for any node $i\in U_{k}$ and any subset $Q \subseteq [n] \setminus \{i\}$.
\end{assumption}

\begin{lemma}
Direct $\mathcal{I}$-Faithfulness assumption is satisfied for the linear SEM with Gaussian noise. More specifically:
\begin{equation*}
    \norm{S_{U_k;i|Q}-S_{i|Q}}_{F}^{2}= \text{fill}  > 0
\end{equation*}
\abhinav{state the condition when it's different}
where $S_{U_k;i|Q}$ is the conditional covariance matrix of node $``i"$ conditioned on set of nodes $Q \subseteq [n] \setminus \{i\}$ for interventional distribution with target set $U_k$ and $S_{i|Q}$ is the observational conditional covariance matrix for node $``i"$ conditioned on $Q$.  
\abhinav{Define similarly for the mean}
\end{lemma}
\begin{proof}
\abhinav{Need to generalize this to arbitrary subset}

\textbf{Case 1}:($Q=[n]\setminus \{i\}, i\in U_k$) The conditional covariance matrix of interventional distribution $f_{U_k}(x_i|\bm{x}_{Q})$ is given by \abhinav{cite the result for gaussian from some textbook}:
\begin{equation}
    S_{U_k; i|Q} = S_{U_k;[i,i]} - S_{U_k;[i,-i]}\Big{(}S_{U_k;[-i,-i]}\Big{)}^{-1}S_{U_k;[-i,i]}
\end{equation}
where where we use the matrix slicing notation to denote $S_{U_k;[i,i]}$ $(i,i)^{\text{th}}$ entry of the interventional covariance matrix $S_{U_k}$, $S_{U_k;[i,-i]}$ denote the $i^{\text{th}}$ row of the $S_{U_k}$ except the $(i,i)$ entry, $S_{U_k;[-i,-i]}$ denote the sub-block of $S_{U_k}$ without the $i^{\text{th}}$ row and column. Using a permutation matrix $P_i$ whose first row is unit vector $\bm{e}_i$, we can write the covariance matrix $S_{U_k}$ as a block matrix of form:
\begin{equation}
    \tilde{S}_{U_k} \triangleq P_i S_{U_k} P_i^{T} = \begin{bmatrix}
        S_{U_k;[i,i]} & S_{U_k;[i,-i]} \\ 
        S_{U_k;[-i,i]} & S_{U_k;[-i,-i]}\\
    \end{bmatrix}
\end{equation}
The $(1,1)^{\text{th}}$ entry of the inverse of the above matrix is equal to the inverse of schur complement of matrix $(\tilde{S}_{U_k})$ i.e:
\begin{equation}
\begin{aligned}
     \Big{(} \tilde{S}_{U_k}/ S_{U_k;[-i,-i]} \Big{)}^{-1} = \frac{1}{S_{U_k; i|Q}} &= \bm{e}_1^{T} \Big{(}\tilde{S}_{U_k}\Big{)}^{-1} \bm{e}_{1}\\
     &= \bm{e}_{1}^{T} \Big{(} P_i S_{U_k}^{-1} P_{i}^{T} \Big{)} \bm{e}_1 \\
     & = \bm{e}_i^{T}\Big{(} (I-A_{U_k})^{T} D_{U_{k}}^{-1} (I-A_{U_k})    \Big{)}\bm{e}_i\\
     &= \frac{1}{\sigma^{'}_{i}} + \sum_{j=i+1}^{n} \frac{1}{\sigma_j}A_{U_k;[j,i]}^{2} \\
\end{aligned}
\end{equation}
\abhinav{Last line is only for atomic intervention i.e $U_{k}=\{i\}$} Similarly (replacing the $U_k$ in the above steps \abhinav{should we write down everything explicitly?}), the conditional covariance of the observational distribution is given by: 
\begin{equation}
\begin{aligned}
     \frac{1}{S_{i|Q}} &= \bm{e}_1^{T} \Big{(}\tilde{S}_{}\Big{)}^{-1} \bm{e}_{1}\\
     &= \bm{e}_{1}^{T} \Big{(} P_i S_{}^{-1} P_{i}^{T} \Big{)} \bm{e}_1 \\
     & = \bm{e}_i^{T}\Big{(} (I-A_{})^{T} D_{}^{-1} (I-A_{})    \Big{)}\bm{e}_i\\
      &= \frac{1}{\sigma_{i}} + \sum_{j=i+1}^{n} \frac{1}{\sigma_j}A_{U_k;[j,i]}^{2} \\
\end{aligned}
\end{equation}
Thus we have:
\begin{equation}
    \Big{|}\frac{1}{S_{U_k; i|Q}} -  \frac{1}{S_{i|Q}}\Big{|} = \Big{|}\frac{1}{\sigma^{'}_{i}} - \frac{1}{\sigma_{i}} \Big{|}\\
\end{equation}
where $\sigma_{i}^{'}\neq \sigma_{i}$.
\end{proof}
\abhinav{Is the set of distribution where the assumption holds. Is it a measure 0, 1 etc, some lower dim space. with prob 1. Adversary will not know the true graph. https://arxiv.org/pdf/1207.0547.pdf.
Karen paper
Jiaqi -- Shift Intervention (Intervention faithfullness)
}

\abhinav{Why we need psi equivalnce if intervention faithfulness holds with pob 1. See  Kaitikeyen paper}

\abhinav{Show it for small graph that we can recover. Give an algorithm}

\abhinav{
\textbf{Next Steps:}
\begin{enumerate}
    \item Finish IMEC result: show for all subsets the covariance and/or mean is different. 
    \item Read $\psi-$MEC paper and connect our result if IMEC needs strong assumptions.
    \item Finish radius of identifiability for non-atomic interventions. 
    \item Generalize to other distribution families: different noise and classes of SEMs.
\end{enumerate}
}
